# Supplementary material for: Many-Body Dephasing by Hole Motion in a Spin-Orbit-Coupled Mott Insulator
Source: arXiv:2409.05828 ancillary file (2024-09-09)
Supplement: Supplementary file 1 [file RamseyMI_SM_v4.pdf]

# Supplementary Material: Many-Body Dephasing by Hole Motion in a Spin-Orbit-Coupled Mott Insulator

Alexis Ghermaoui,[1] Manel Bosch Aguilera,[1] Raphaël Bouganne,[1] Rémy Vatré,[1] Isabella Fritsche,[2,3] Jérôme Beugnon,[1] and Fabrice Gerbier[1,*]

[1]*Laboratoire Kastler Brossel, Collège de France, CNRS, ENS-Université PSL, Sorbonne Université, 11 place Marcelin Berthelot, F-75231 Paris, France*

[2]*Institut für Quantenoptik und Quanteninformation (IQOQI), Österreichische Akademie der Wissenschaften, 6020 Innsbruck, Austria*

[3]*Institut für Experimentalphysik, Universität Innsbruck, 6020 Innsbruck, Austria*

(Dated: September 8, 2024)

## A LASER-DRIVEN TWO-COMPONENT QUANTUM GAS IN AN OPTICAL LATTICE

### Hamiltonian and notations

We consider a many-body system of atoms with two internal states labeled $\sigma = \downarrow, \uparrow$. With a slight abuse of notations, we denote with $\sigma$ the internal state labels or their "signature" $\sigma = \pm 1$ for $\uparrow, \downarrow$. We note $\hat{a}_{m,\sigma}$ the annihilation operator of a bosons at site $m$ in spin state $\sigma$. We recall for completeness the definition of the local spin operators,

$$\hat{\boldsymbol{s}}_m = \begin{pmatrix} \frac{1}{2}\left(\hat{s}_{m,+} + \hat{s}_{m,-}\right) \\ \frac{1}{2\mathrm{i}}\left(\hat{s}_{m,+} - \hat{s}_{m,-}\right) \\ \frac{1}{2}\left(\hat{a}^\dagger_{m,\uparrow}\hat{a}_{m,\uparrow} - \hat{a}^\dagger_{m,\downarrow}\hat{a}_{m,\downarrow}\right) \end{pmatrix}. \quad (1)$$

with the spin raising and lowering operators $\hat{s}_{m,+} = \hat{a}^\dagger_{m,\uparrow}\hat{a}_{m,\downarrow}$ and $\hat{s}_{m,-} = \left(\hat{s}_{m,+}\right)^\dagger$, respectively. The global spin operators are noted with upper case letters, *e.g.* $\hat{S}_\alpha = \sum_m \hat{s}_{m,\alpha}$ with $\alpha = x, y, z$.

We recall the many-body Hamiltonian

$$\widetilde{H} = \widetilde{H}_0 - \hbar\delta_{\mathrm{L}}\hat{S}_z + f(t)\widetilde{V}_{\mathrm{L}}. \quad (2)$$

The motional Hamiltonian $\widetilde{H}_0 = \widetilde{K} + \hat{H}_{\mathrm{int}}$ is the sum of the single-particle and interaction Hamiltonians $\widetilde{K}$ and $\hat{H}_{\mathrm{int}}$, respectively. For simplicity, we consider a one-dimensional system in the fundamental band of a deep lattice in the tight binding regime. We note $\langle x|w_m\rangle = w(x - x_m)$ the one-dimensional Wannier function of the fundamental band localized around site $m$ located at $x_m = md$, and $W$ its three-dimensional counterpart. The single-particle Hamiltonian is

$$\widetilde{K} = -t_{\mathrm{nn}} \sum_{m,\sigma=\uparrow,\downarrow} \hat{a}^\dagger_{m+1,\sigma}\hat{a}_{m,\sigma} + \mathrm{h.c.}, \quad (3)$$

with $t_{\mathrm{nn}}$ the nearest-neighbor tunneling energy. As in the main text, we assume that the interaction Hamiltonian is invariant by spin rotations, *i.e.* $\left[\hat{H}_{\mathrm{int}}, \hat{S}_\alpha\right] = 0$ with $\alpha = \pm, z$.

The other two terms describe the internal dynamics, with the coupling term $\widetilde{V}_{\mathrm{L}}$ describing the electric dipole interaction Hamiltonia between each atom and a monochromatic laser wave inducing transitions between the two internal states. We write the laser electrric field $\boldsymbol{E}_{\mathrm{L}}(\boldsymbol{r}, t) = \mathcal{E}_{\mathrm{L}} \cos\left(\boldsymbol{k}_{\mathrm{L}} \cdot \boldsymbol{r} + \phi - \omega_L t\right)\boldsymbol{e}_y$, with $\omega_{\mathrm{L}}, k_{\mathrm{L}}, \mathcal{E}_{\mathrm{L}}, \phi$ the laser frequency, wavevector, amplitude and global phase, respectively. We make the rotating wave approximation (*e.g.*, [1]) and neglect the excited bands and the spatial overlap integrals for different sites $m' \neq m$. The electric dipole coupling Hamiltonian then reads

$$\widetilde{V}_L = -\hbar\Omega \sum_m \hat{\boldsymbol{s}}_m \cdot \boldsymbol{v}_m, \quad (4)$$

with a local axis

$$\boldsymbol{v}_m = \cos\left(mk_{\mathrm{L}}d + \phi\right)\boldsymbol{e}_y - \sin\left(mk_{\mathrm{L}}d + \phi\right)\boldsymbol{e}_x \quad (5)$$

and a renormalized Rabi frequency,

$$\Omega = \Omega_{\mathrm{L}} \int \mathrm{d}^3\boldsymbol{r'}\, |W(\boldsymbol{r'})|^2 \cos\left(\boldsymbol{k}_{\mathrm{L}} \cdot \boldsymbol{r'}\right), \quad (6)$$

*i.e.* the free space Rabi frequency $\Omega_{\mathrm{L}}$ corrected by a *Lamb-Dicke factor* [2].

### Ramsey interferometer in the lab frame: Spin spiral state

As discussed in the main text, the evolution operators during the $\pi/2$ pulses are well approximated by

$$\mathrm{e}^{-\mathrm{i}\frac{t}{\hbar}\widetilde{V}_{\mathrm{L}}(\phi)} = \prod_m \mathrm{e}^{\mathrm{i}\frac{\Omega t}{2}\hat{\boldsymbol{s}}_m \cdot \boldsymbol{v}_m}, \quad (7)$$

a product of individual on-site rotation operators with the same rotation angle $-\Omega t/2$ for all sites but a site-dependent rotation axis $\boldsymbol{v}_m$ due to the recoil phase. In this work,we always consider Ramsey sequences with an initial state prepared in the $\downarrow$ manifold. The first (preparation) $\pi/2$ pulse with $\phi = 0$ corresponds to local rotation operators $\hat{R}_1^{(m)} = \mathrm{e}^{\mathrm{i}\frac{\pi}{2}\hat{\boldsymbol{s}}_m \cdot \boldsymbol{v}_m}$ mapping the $-\boldsymbol{e}_z$ axis to

$$\boldsymbol{u}_m = \cos\left(mk_{\mathrm{L}}d\right)\boldsymbol{e}_x + \sin\left(mk_{\mathrm{L}}d\right)\boldsymbol{e}_y, \quad (8)$$

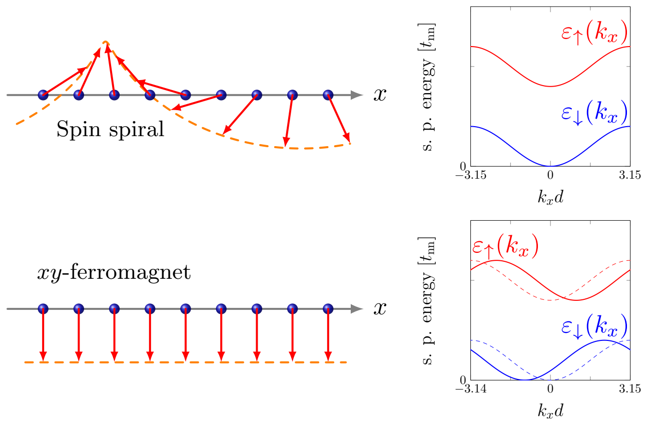


FIG. S1. Illustration of the two equivalent pictures used: in the lab frame, the initial state is a spin spiral with a pitch determined by the recoil phase. The dispersion relations are identical for each spin state up to an overall energy shift. In the spiral frame, the initial state is polarized along the same direction for every site. The recoil phase is transferred tothe single-particle dispersion relations which now have different minima.

and the initial $|\downarrow\rangle_m$ state to

$$|+\boldsymbol{u}_m\rangle = \hat{R}_1^{(m)}|\downarrow\rangle_m \quad = \frac{1}{\sqrt{2}}\left(|\downarrow\rangle_m + \mathrm{e}^{-\mathrm{i}mk_\mathrm{L}d}|\uparrow\rangle_m\right), \tag{9}$$

the eigenstate of the operator $\hat{\boldsymbol{s}}_m \cdot \boldsymbol{u}_m$ with eigenvalue $+1/2$ . For the second (read-out) $\pi/2$ pulse, the local rotation axis become

$$\boldsymbol{u}'_m = \cos\phi\boldsymbol{u}_m + \sin\phi\boldsymbol{v}_m, \tag{10}$$
$$\boldsymbol{v}'_m = -\sin\phi\boldsymbol{u}_m + \cos\phi\boldsymbol{v}_m, \tag{11}$$

with the relative phase $\phi$ controlling the mismatch between the preparation and read-out axis.

We now discuss the experimental situation where the initial state is a Mott insulator state with one atom in the $\downarrow$ state at each site. The preparation $\pi/2$ pulse transforms the $\downarrow$-polarized Mott insulator into a so-called *spin spiral state* $|\text{spin spiral}\rangle = \prod_m |+\boldsymbol{u}_m\rangle_m$, where the mean spin vector is completely polarized (maximum modulus 1/2) but the polarization axis is parallel to $\boldsymbol{u}_m$ and therefore rotates along the chain with a period $2\pi/\eta$ (see Fig. S1a). Changing the overall phase to $\phi \neq 0$ only shifts the spiral without affecting its structure.

The dynamics of such spin spiral structures [3, 4] has been investigated in several previous experiments with (pseudo-)spin 1/2 bosonic and fermionic quantum gases of alkali atoms [5–10]. In these experiments, the two spin states were the two hyperfine states in the ground electronic manifold. Coupling two such hyperfine states with one-photon transitions requires radio-frequency or microwave radiation, where $2\pi/k_\mathrm{L}$ is very large and recoil is negligible. To create a spin spiral state, the atoms are held in an applied magnetic field gradient right after the preparation $\pi/2$ pulse. In our experiments, the spiral structure comes naturally with the spin-orbit coupling associated with the recoil momentum. A key feature is that an identical spiral structure (up to the global shift controlled by $\phi$) is imprinted by the preparation pulse *and* by the readout pulses. Note that this also applies for alkali atoms if two-photon Raman transitions are used instead of one-photon transitions.

### Ramsey interferometer in the spiral frame: Spin-orbit coupling

As stated in the main article, it is convenient to make a "unitary transformation to the spiral frame" defined by the operator

$$\hat{\mathcal{T}}_2 = \mathrm{e}^{-\mathrm{i}\sum_m \boldsymbol{k}_\mathrm{L}\cdot\boldsymbol{r}_m \hat{s}_{m,z}}, \tag{12}$$

a rotation along $\boldsymbol{z}$ with a site-dependent angle to "unwind" the spin spiral. The annihilation operators transform as $\hat{\mathcal{T}}_2 \hat{a}_{m,\sigma}\hat{\mathcal{T}}_2^\dagger = \mathrm{e}^{\mathrm{i}\sigma\frac{\boldsymbol{k}_\mathrm{L}\cdot\boldsymbol{r}_m}{2}}\hat{a}_{m,\sigma}$, and the kinetic and electric dipole Hamiltonians become respectively Eq. (1) in the main article and

$$\hat{V}_\mathrm{L} = \hat{\mathcal{T}}_2 \widetilde{V}_\mathrm{L} \hat{\mathcal{T}}_2^\dagger = -\hbar\Omega\hat{\boldsymbol{S}}\cdot\boldsymbol{v}(\phi), \tag{13}$$

with the unit vector $\boldsymbol{v}(\phi) = -\sin\phi\boldsymbol{e}_x + \cos\phi\boldsymbol{e}_y$ is now the same for all sites. After the first Ramsey pulse, an initial Fock state $\left|\downarrow\right\rangle_m$ becomes $\hat{R}_1\left|\downarrow\right\rangle_m = \left|+\boldsymbol{x}\right\rangle_m$, the eigenstate of $\boldsymbol{s}_{m,x}$ with eigenvalue $+1/2$ (see Fig. S1b). The corresponding annihilation operator is $\hat{a}_{m,\pm\boldsymbol{x}} = \left(\hat{a}_{m,\uparrow} \pm \hat{a}_{m,\downarrow}\right)/\sqrt{2}$.

## RAMSEY SIGNAL

In this Section, we give the details of the derivation of the formula for the Ramsey signal [Eq. (6) in the main text]. We work within the rotating wave approximation and in the spiral frame discussed in Section . We note $\hat{R}_1 \equiv \hat{R}_{\boldsymbol{e}_y}(-\pi/2)$, $\hat{R}_2(\phi) \equiv \hat{R}_{\boldsymbol{v}(\phi)}(-\pi/2)$ the evolution operators corresponding to the preparation and read-out $\pi/2$ pulses. In the spin echo case, we choose to apply the $\pi-$pulse along the same axis as the first rotation, so that the corresponding evolution operator is $\hat{R}_\pi = \hat{R}_1^2$.

### Without spin echo

We first consider the two-axis Ramsey sequence without spin echo. The total evolution operator reads $\hat{U}_\mathrm{total} = \hat{R}_2(\phi)\hat{U}(T)\hat{R}_1$ , where $\hat{U}(T)$ describes the many-body dynamics between the pulses. Using $[\hat{H}_0, \hat{S}_z] = 0$, we

write $\hat{U}(T) = \mathrm{e}^{\mathrm{i}\zeta \hat{S}_z}\hat{U}_0(T)$, with the Larmor phase $\zeta(t) = \int_0^t \delta_{\mathrm{L}}(t')dt'$ and with the "free evolution" operator

$$\hat{U}_0(T) = \mathrm{e}^{-\mathrm{i}\frac{\hat{H}_0 T}{\hbar}}. \tag{14}$$

The Ramsey signal

$$\mathcal{R}(\phi, T) = \frac{1}{2} - \frac{1}{N}\sum_m \left\langle \Psi_{\mathrm{ref}} \middle| \hat{U}_0^\dagger(T)\hat{s}'_{m,z}\hat{U}_0(T) \middle| \Psi_{\mathrm{ref}} \right\rangle \tag{15}$$

is the expectation value of the counter-rotated final observable that takes into account the read-out pulse and the Larmor precession during $T$,

$$\begin{aligned} \hat{s}'_{m,z} &= \mathrm{e}^{-\mathrm{i}\zeta \hat{S}_z}\hat{R}_2(\phi)^{'\dagger}\hat{s}_{m,z}\hat{R}_2(\phi)\mathrm{e}^{\mathrm{i}\zeta \hat{S}_z}, \\ &= \cos(\zeta - \phi)\hat{s}_{m,x} + \sin(\zeta - \phi)\hat{s}_{m,y}, \end{aligned} \tag{16}$$

in the state time-evolved from the rotated initial state $|\Psi_{\mathrm{ref}}\rangle = \hat{R}_1|\Psi_{\mathrm{i}}\rangle$ ("reference state" thereafter) . We thus find that the Ramsey signal is given by

$$\begin{aligned} \mathcal{R}(\phi, T) = \frac{1}{2} - \frac{1}{N}\sum_m & \cos(\phi - \zeta)\,\langle \hat{s}_{m,x}\rangle_T \\ & + \sin(\phi - \zeta)\,\langle \hat{s}_{m,y}\rangle_T, \end{aligned} \tag{17}$$

where the spin expectation values ($\alpha = x, y$)

$$\langle \hat{s}_{m,\alpha}\rangle_T = \langle \Psi_{\mathrm{ref}}|\hat{U}_0(T)^\dagger\, \hat{s}_{m,\alpha}\, \hat{U}_0(T)|\Psi_{\mathrm{ref}}\rangle, \tag{18}$$

are computed with the "laser-free" many-body evolution operator $\hat{U}_0$.

### With spin echo

With an additional spin echo pulse inserted in the middle of the Ramsey sequence, the total evolution operator becomes $\hat{U}_{\mathrm{total}} = \hat{R}_2(\phi)\,\hat{U}_2(T/2)\hat{R}_\pi\hat{U}_1(T/2)\,\hat{R}_1$, with $\hat{U}_\alpha(T/2) = \mathrm{e}^{\mathrm{i}\zeta_\alpha \hat{S}_z}\hat{U}_0(T/2)$ the evolution operators for the periods $\alpha = 1, 2$, and $\zeta_1 = \int_0^{T/2}\delta_{\mathrm{L}}(t')dt'$, $\zeta_2 = \int_{T/2}^{T}\delta_{\mathrm{L}}(t')dt'$ the corresponding Larmor phases. We rearrange the expression for the total evolution operator as

$$\hat{U}_{\mathrm{total}} = -\Big(\hat{R}_2(\phi)\mathrm{e}^{\mathrm{i}(\zeta_2-\zeta_1)\hat{S}_z}\Big)\,\cdot\,\hat{U}_{\mathrm{SE}}\,\cdot\,\hat{R}_1,$$

where we used the operator identity $\hat{R}_1^2\mathrm{e}^{\mathrm{i}\zeta_1\hat{S}_z} = -\mathrm{e}^{-\mathrm{i}\zeta_1\hat{S}_z}\hat{R}_1^2$ and defined a spin echo evolution operator

$$\hat{U}_{\mathrm{SE}} = \hat{U}_0(T/2)\hat{R}_\pi\hat{U}_0(T/2). \tag{19}$$

The total evolution operator has the same global structure as for the sequence without spin echo up to the replacements $\hat{U}_0(T) \longrightarrow \hat{U}_{\mathrm{SE}}$ and $\zeta \longrightarrow \zeta_2 - \zeta_1$. The Ramsey signal is then

$$\begin{aligned} \mathcal{R}_{\mathrm{SE}}(\phi, T) = \frac{1}{2} + \frac{1}{N}\sum_m & \cos(\phi - \zeta_2 + \zeta_1)\,\langle \hat{s}_{m,x}\rangle_T \\ & + \sin(\phi - \zeta_2 + \zeta_1)\,\langle \hat{s}_{m,y}\rangle_T, \end{aligned} \tag{20}$$

where the spin expectation values ($\alpha = x, y$) are now given by Eq. (18) with the replacement $\hat{U}_0 \longrightarrow \hat{U}_{\mathrm{SE}}$. If we neglect frequency fluctuations of the laser, the two Larmor phases become equal, $\zeta_1 = \zeta_2 = \delta_{\mathrm{L}}T/2$.

## INFLUENCE OF THE LASER FREQUENCY NOISE

### General formula

Experimentally, fluctuations of the driving laser frequency can be a significant detrimental factor reducing the Ramsey fringe contrast. Understanding their effect in details is crucial to be able to distinguish the dephasing due to laser fluctuations from the intrinsic dephasing dynamics we aim to study. To that aim, we write the time-dependent laser frequency as $\omega_{\mathrm{L}}(t) = \overline{\omega}_{\mathrm{L}} + \delta\omega_{\mathrm{L}}(t)$, where the frequency noise $\delta\omega_{\mathrm{L}}$ is taken to be a Gaussian stationary stochastic variable with zero mean. The Larmor phase $\zeta(t) = \overline{\zeta} + \delta\zeta(t)$ thus features a deterministic component $\overline{\zeta} = \delta_{\mathrm{L}}t$ determined by the average detuning $\delta_L = \overline{\omega}_{\mathrm{L}} - \omega_0$, and a stochastic component given by the integrated frequency noise, $\delta\zeta = \int_0^t \delta\omega_L(t')dt'$. After statistical averaging over the noise (denoted by the upper bar), we find for the two-axis sequence without spin echo

$$\begin{aligned} \overline{\mathcal{R}}(\phi, T) = \frac{1}{2} - \mathrm{e}^{-F(T)}\sum_m & \cos(\phi - \overline{\zeta})\,\langle \hat{s}_{m,x}\rangle \\ & + \sin(\phi - \overline{\zeta})\,\langle \hat{s}_{m,y}\rangle. \end{aligned} \tag{21}$$

The noise factor $F = \overline{\delta\zeta^2}/2$ is determined by the laser frequency fluctuations and the pulse length and shape. The same reasoning in the case with spin echo leads to

$$\begin{aligned} \overline{\mathcal{R}}_{\mathrm{SE}}(\phi, T) = \frac{1}{2} + \mathrm{e}^{-F_{\mathrm{SE}}(T)}\sum_m & \cos(\phi)\,\langle \hat{s}_{m,x}\rangle \\ & + \sin(\phi)\,\langle \hat{s}_{m,y}\rangle, \end{aligned} \tag{22}$$

where $F_{\mathrm{SE}}(T) = \overline{(\zeta_2 - \zeta_1)^2}/2$ is the stochastic mean square average of the differential Larmor phase accumulated after the two Ramsey half-periods, and where the spin expectation values are computed with the spin echo evolution operator in Eq. (19).

Assuming that the frequency noise is a stationary process obeying the Wiener-Khintchin theorem, we find after some algebra that the noise factor can be expressed as

$$\left.\begin{matrix} F(T) \\ F_{\mathrm{SE}}(T) \end{matrix}\right\} = \int_{-\infty}^{+\infty}\frac{d\Omega}{2\pi}\,S_{\delta\omega_{\mathrm{L}}}(\Omega)\left\{\begin{matrix} W(\Omega, T) \\ W_{\mathrm{SE}}(\Omega, T) \end{matrix}\right., \tag{23}$$

with $S_{\delta\omega_{\mathrm{L}}}$ the laser frequency noise spectral density and

with the window functions

$$W(\Omega,T) = \frac{T^2}{2}\frac{\sin^2\left(\frac{\Omega T}{2}\right)}{\left(\frac{\Omega T}{2}\right)^2}, \tag{24}$$

$$W_{\mathrm{SE}}(\Omega,T) = \frac{T^2}{2}\frac{\sin^4\left(\frac{\Omega T}{4}\right)}{\left(\frac{\Omega T}{4}\right)^2} \tag{25}$$

in the case without or with spin echo, respectively.

### Influence of the laser frequency noise spectrum

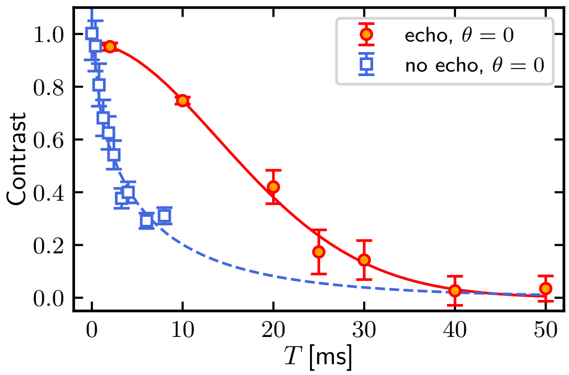


FIG. S2. Decay of the Ramsey fringe contrast for $V_x = 26\,E_{\mathrm{R}}$. The two different incidence angles $\theta = 0, \pi/4$ of the coupling laser correspond to recoil phases $\eta = \pi \times 1.31$ or 0.92, respectively.

The window functions act as frequency filters restricting the range of contributing frequencies to a particular window, either to frequencies $\Omega \lesssim 2\pi/T$ without spin echo, or to a narrower window centered around $2\pi/T$ with spin echo. When the noise spectral density behaves as a power law $S_{\delta\omega_{\mathrm{L}}}(\Omega) \approx S_0(\Delta\Omega/\Omega)^\alpha$ in the relevant frequency window, one finds

$$F_{2\mathrm{A}/\mathrm{SE}}(T) \simeq S_0\Delta\Omega^\alpha T^{\alpha+1}\int_0^{+\infty}\frac{p^{1-\alpha}\sin^p u}{u^{2+\alpha}}du, \tag{26}$$

where $p = 2$ without spin echo (2A) and $p = 4$ with spin echo (SE). We assume here that the integral over $[0, +\infty[$ converges. In the opposite case, the noise spectrum in the relevant frequency window cannot be described by a simple power law.

Two particular cases are of special interest. A frequency-independent ("white") noise spectrum gives a linear increase of the noise factor with time,

$$F_{2\mathrm{A}/\mathrm{SE}}(T) \underset{\text{white noise}}{\simeq} \pi\, S_0\, T, \tag{27}$$

and consequently an exponential decay of the fringe contrast. A noise spectrum decaying as $1/\Omega$ ("frequency flicker" noise) gives instead a quadratic increase of the noise factor with time,

$$F_{\mathrm{SE}}(T) \underset{\text{flicker noise}}{\simeq} \ln 2 \cdot S_0 \cdot \Delta\Omega \cdot T^2, \tag{28}$$

and consequently a Gaussian decay of the fringe contrast.

### Experimental results

We perform Ramsey experiments with and without spin echo for atoms trapped by a deep lattice with $V_{0x/y/z} = 26\,E_{\mathrm{R}}$. In this situation, atomic motion by tunneling is negligible over the course of the sequence and the dephasing of the Ramsey fringe is entirely determined by the laser noise. The experimental results shown in Fig. S2 show a dephasing time an order of magnitude larger with spin echo than without. A fit to the data with a function of the form $C_0 \exp\left[-(\gamma t)^\alpha\right]$ returns an almost exponential behavior without spin echo (best fit parameter $\alpha \approx 0.9(2)$, where the error bar denotes the $1/e$ confidence interval of the fit) and an almost Gaussian behavior with spin echo [$\alpha \approx 1.9(2)$]. Fixing the exponents to $\alpha = 1$ and 2, we extract experimental decay rates $\gamma_1 \approx 260(30)\,\mathrm{s}^{-1}$ and $\gamma_2 \approx 49(3)\,\mathrm{s}^{-1}$ without and with spin echo, respectively.

The experimental observations point to a noise spectrum of the kind sketched in Fig. S3, with a "flicker" noise $\Omega^{-1}$ behavior at low frequencies and a white noise behavior at high frequencies and a characteristic frequency $\omega_1 \simeq \Delta\Omega$ separating the two limiting behavior. Experimental data without spin echo end up in the regime $\omega_1 T \ll 1$ where the white noise floor prevails. Experimental data with spin echo probe instead the flicker noise regime $\omega_1 T \gg 1$. This scenario is compatible with the measurement if $\omega_1/(2\pi)$ is on the order of a few tens of Hz. From the fitted $\gamma_1$ and Eq. (27), we extract a value $S_0 = \gamma_1/\pi \approx 83(9)\,\mathrm{s}^{-1}$. From the fitted $\gamma_2$ and Eq. (28), we extract a value $\Delta\Omega \approx 40(5)\,\mathrm{s}^{-1}$.

## CALCULATION OF THE RAMSEY SIGNAL FOR HARDCORE BOSONS

### Hardcore bosons with two internal components

We consider hardcore bosons defined by the relation $a_{i,\sigma}a_{i,\sigma'} = 0$ (and its conjugate), which forces the local occupation numbers to be 0 or 1. The Hamiltonian $\hat{H}_0$ reduces to the single particle term in Eq. (1,9) of the main article,

$$\hat{K} = \sum_{m,\sigma=\pm\boldsymbol{x},d=\pm 1} -\overline{W}\hat{a}^\dagger_{m+d,\sigma}\hat{a}_{m,\sigma} + \mathrm{i}\,dW_{\mathrm{SO}}\hat{a}^\dagger_{m+d,-\sigma}\hat{a}_{m,\sigma}, \tag{29}$$

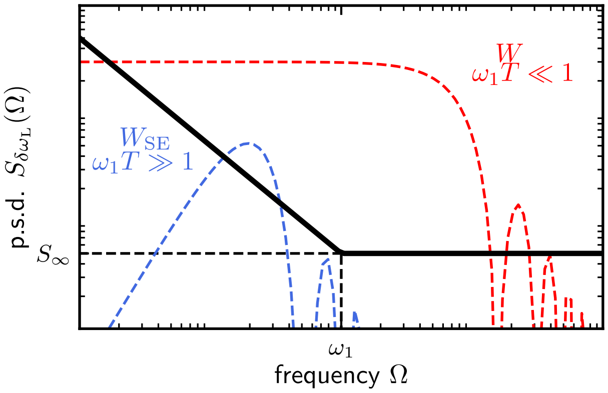


FIG. S3. Sketch of the power spectrum with a "flicker" noise $\Omega^{-1}$ behavior at low frequencies and a white noise behavior at high frequencies (solid black line). The blue dashed and red dash-dotted lines show the window functions for Ramsey sequences with or without spin echo, respectively.

with $\overline{W} = t_{\rm nn}\cos(k_0 d/2)$ and $W_{\rm SO} = t_{\rm nn}\sin(k_0 d/2)$. In the one-component case, a Jordan-Wigner transformation can be used to map to a free fermionic problem (although computing the original bosonic observables is usually rather complicated due to the occupation-number-dependent phase factors which come with this transformation). For a two-component system, the Jordan-Wigner-transformed Hamiltonian does not take a simple quadratic form.

## Perturbative calculations

Without loss of generality, in this Section, we take $\delta_{\rm L} = 0$, $\phi = 0$ and ignore the laser frequency fluctuations. The Ramsey signal is then given by $\mathcal{R}_{\rm SE}(\phi, T) = [1 + C(T)]/2$ and the contrast by $C(T) = 2\left|\langle \hat{S}_x\rangle\right|/N$. We denote by "reference state" the fully polarized state with exactly one atom per site,

$$|\Psi_{\rm ref}\rangle = \prod_m \hat{a}^\dagger_{m,+\boldsymbol{x}}|\varnothing\rangle. \tag{30}$$

Since $\hat{K}|\Psi_{\rm ref}\rangle = 0$, the Ramsey contrast never changes irrespective of the sequence used. The freezing of atomic motion by interactions completely suppresses spin-orbit-induced dephasing. We have to consider at least one unoccupied site to observe an effect. This calculation is performed below. For the sake of comparison, we also calculate with the same method what happens for the single-particle state $\big| +\boldsymbol{x}\big\rangle_m$ .

### *Perturbative calculation*

We first derive perturbative formulas for the expectation value of an observable, $\langle \hat{O}\rangle = \langle \Psi(t)|\hat{O}|\Psi(t)\rangle$, with the time-evolved state $|\Psi(t)\rangle = \exp(-{\rm i}\hat{H}_0 t/\hbar)|\Psi(0)\rangle$ expanded to second order in time. For the Ramsey signal, we take $\hat{O} = \hat{S}_x$ but keep the notation general for the time being. We call $(\{|\phi_j\rangle, o_j\}$ the eigenstates and eigenvalues of $\hat{O}$, such that $\hat{O}|\phi_j\rangle = o_j|\phi_j\rangle$, and assume that the initial state $|\Psi(0)\rangle \equiv |\phi_0\rangle$ is one of the eigenvectors with eigenvalue $o_0$. For the Ramsey sequence with spin echo, we also assume that any eigenstate of $\hat{O}$ remains an eigenstate (not necessarily the same) after a $\pi$ pulse, *i.e.* $\hat{O}|\phi'_j\rangle = o'_j|\phi'_j\rangle$ with $|\phi'_j\rangle = \hat{R}_\pi|\phi_j\rangle$. After some algebra , we find

$$\langle\hat{O}\rangle \simeq o_0 - \left(\frac{t}{\hbar}\right)^2 \sum_j (o_0 - o_j)\left|\langle\phi_j|\hat{H}_0|\phi_0\rangle\right|^2 + \cdots \tag{31}$$

without spin echo, and

$$\langle\hat{O}\rangle \simeq o'_0 - \left(\frac{t}{2\hbar}\right)^2 \sum_j (o'_0 - o'_j)\times \left|\langle\phi_j|\hat{H}_0|\phi_0\rangle + \langle\phi_j|\hat{R}^\dagger_\pi\hat{H}_0\hat{R}_\pi|\phi_0\rangle\right|^2 \tag{32}$$

with spin echo. In both cases, only spin-changing tunneling processes $\propto W_{\rm SO}$ contribute to the dephasing of the Ramsey signal due to the weight factors $o_j - o_0$ in Eqs. (31,32). In the spin echo case, the direct $\langle\phi_j|\hat{H}_0|\phi_0\rangle$ and "$\pi$-transformed" $\langle\phi_j|\hat{R}^\dagger_\pi\hat{H}_0\hat{R}_\pi|\phi_0\rangle$ transition amplitudes must be added coherently.

*One particle:* We treat first the case of a single particle localized initially at site $m_0$, $|\phi_0\rangle = \hat{a}^\dagger_{m_0,+\boldsymbol{x}}|\varnothing\rangle$. Without spin echo, Eq. (31) yields

$$C(T) \simeq 1 - \left(\frac{2W_{\rm SO}T}{\hbar}\right)^2. \tag{33}$$

In this simple case, the problem can also be solved exactly in momentum space [11], leading to $C(T) = J_0\left(4W_{\rm SO}T/\hbar\right)$. Using the Taylor expansion $J_0(x) \approx 1 - x^2/4$, we recover Eq. (33).

With spin echo, the direct and $\pi-$reversed amplitudes have opposite signs, $\langle\phi_j|\hat{H}_0|\phi_0\rangle = {\rm i}W_{\rm SO} = -\langle\phi_j|\hat{R}^\dagger_\pi\hat{H}_0\hat{R}_\pi|\phi_0\rangle$, and therefore interfere destructively in Eq. (32). The spin average after spin echo is then undamped,

$$C_{\rm SE}(T) \simeq 1 + \mathcal{O}(\tau^3),$$

in agreement with the exact result $C_{\rm SE}(T) = 1$ [11].

*One hole:* We now consider an initial state with one atom per site everywhere, except for a single hole at site $m_0$, $|\phi_0\rangle = |{\rm h} : m_0\rangle = \hat{a}_{m_0,+\boldsymbol{x}}|\Psi_{\rm ref}\rangle$. This state is an eigenvector of $\hat{S}_x$ with eigenvalue $o_0 = (N_s - 1)/2$. The action of the Hamiltonian on $|\phi_0\rangle$ is

$$\hat{H}_0|\phi_0\rangle = \sum_{d=\pm1} -\bar{W}|{\rm h} : m_0 + d\rangle + + {\rm i}dW_{\rm SO}\hat{a}^\dagger_{m_0,-\boldsymbol{x}}\hat{a}_{m_0,+\boldsymbol{x}}|{\rm h} : m_0 + d\rangle. \tag{34}$$

The first term $\propto \bar{W}$ corresponds to a one-hole state with the hole at a different position $m_0 \pm 1$. The second term $\propto W_{\rm SO}$ with an additional spin-flip "defect" at the original hole position $m_0$ determines the decay of the Ramsey signal. Using again Eq. (31) with $\hat{O} = \hat{S}_x$, we obtain

$$C(T) \simeq 1 - \frac{1}{N_s - 1}\left(\frac{2W_{\rm SO}T}{\hbar}\right)^2. \qquad (35)$$

For the spin echo sequence, the transition amplitudes for the one-hole state or for its $\pi-$ transformed analog are equal in magnitude, $\langle\phi_j|\hat{H}_0|\phi_0\rangle = \langle\phi_j|\hat{R}_\pi^\dagger \hat{H}_0 \hat{R}_\pi|\phi_0\rangle = {\rm i}\,W_{\rm SO}$, and therefore interfere *constructively* unlike in the one-particle case. The contrast decay is then the same with or without spin echo,

$$C_{\rm SE}(T) = C(T) \simeq 1 - \frac{1}{N_s - 1}\left(\frac{2W_{\rm SO}T}{\hbar}\right)^2. \qquad (36)$$

**Exact numerical calculations for $N = 12$ sites**

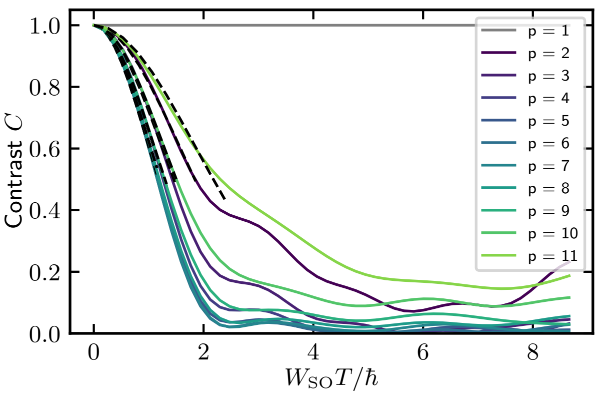


FIG. S4. Numerical simulations for $p$ hardcore bosons in a one-dimensional lattice with $N_s = 12$ sites. The black dashed lines show the Gaussian fits for $C \geq 0.5$. We use $\eta = 4\pi/3$ and periodic boundary conditions.

In order to go beyond the perturbative results, we perform calculations with $p$ hardcore particles on a lattice with $N_s$ sites. The Hilbert space is spanned by Fock states of the form

$$|\boldsymbol{m}, \boldsymbol{\sigma}\rangle = \prod_{i=1}^{p} \hat{a}^\dagger_{m_i,\sigma_i}|\varnothing\rangle, \qquad (37)$$

where $|\varnothing\rangle$ denotes the vacuum state. The total number of Fock states is $\binom{N_s}{p} \times 2^p$. The rotation operator $\hat{R}_{\boldsymbol{n}}^{(m)}(\alpha)$ of angle $\alpha$ around the axis $\boldsymbol{v}$ for hardcore bosons is

$$\hat{R}_{\boldsymbol{n}}^{(m)}(\alpha) = \hat{P}_0^{(m)} + \hat{P}_1^{(m)}\left[\cos\frac{\alpha}{2} - {\rm i}\,\sin\frac{\alpha}{2}\hat{\sigma}_m\cdot\boldsymbol{v}\right]\hat{P}_1^{(m)}, \qquad (38)$$

with $\hat{\sigma}_m = 2\hat{s}_m$ a Pauli matrix, and with $\hat{P}_0^{(m)} = 1 - \hat{n}_m$ and $\hat{P}_1^{(m)} = \hat{n}_m$ the projectors on the subspace with zero and unity occupation at site $m$, respectively. The rotation operators mix the internal quantum numbers $\boldsymbol{\sigma}$, without affecting the motional quantum numbers $\boldsymbol{m}$. As a result, one can write

$$\hat{R}_1|\boldsymbol{m},\boldsymbol{\sigma}\rangle = \sum_{\boldsymbol{\sigma'}} \alpha^{(\boldsymbol{m})}_{\boldsymbol{\sigma},\boldsymbol{\sigma'}}|\boldsymbol{m},\boldsymbol{\sigma'}\rangle, \qquad (39)$$

$$\hat{R}_\pi|\boldsymbol{m},\boldsymbol{\sigma}\rangle = \sum_{\boldsymbol{\sigma'}} \beta^{(\boldsymbol{m})}_{\boldsymbol{\sigma},\boldsymbol{\sigma'}}|\boldsymbol{m},\boldsymbol{\sigma'}\rangle. \qquad (40)$$

where the matrices $\alpha^{(\boldsymbol{m})}, \beta^{(\boldsymbol{m})}$ can be calculated analytically. On the opposite, the tunneling operator mixes the motional quantum numbers $\boldsymbol{m}$ but cannot alter the internal state configuration $\boldsymbol{\sigma}$. The Hamiltonian $\hat{H}_0$ is therefore block diagonal with a given block of size $\binom{N_s}{p}$ corresponding to a particular spin configuration $\boldsymbol{\sigma}$. The evolution operator during the Ramsey period is thus of the form

$$\hat{U}_0(T/2) = {\rm e}^{-{\rm i}\frac{\hat{H}_0 T}{2\hbar}}|\boldsymbol{m},\boldsymbol{\sigma}\rangle = \sum_{\boldsymbol{m'}} \gamma^{(\boldsymbol{\sigma})}_{\boldsymbol{m},\boldsymbol{m'}}|\boldsymbol{m'},\boldsymbol{\sigma}\rangle, \qquad (41)$$

where the matrix $\gamma^{(\boldsymbol{\sigma})}$ is calculed numerically from the eigenstates and eigenvalues of $\hat{H}_0$.

We perform calculations in the lab frame with an initial Fock state $|\Psi_0\rangle = |\boldsymbol{m}_0, \boldsymbol{\sigma}_0\rangle$, where the entries of $\boldsymbol{m}_0$ are zero except for $p$ occupied sites, and where the entries of $\boldsymbol{\sigma}_0$ are $\downarrow$. The many body state at the end of the Ramsey sequence is then

$$|\Psi(T)\rangle = \hat{U}_{\rm SE}\hat{R}_1|\boldsymbol{m}_0, \boldsymbol{\sigma}_0\rangle, \qquad (42)$$

with the spin echo evolution operator

$$\langle\boldsymbol{m'},\boldsymbol{\sigma'}|\hat{U}_{\rm SE}|\boldsymbol{m},\boldsymbol{\sigma}\rangle = \sum_{\boldsymbol{m}_1} \gamma^{(\boldsymbol{\sigma'})}_{\boldsymbol{m}_1,\boldsymbol{m'}}\beta^{(\boldsymbol{m}_1)}_{\boldsymbol{\sigma},\boldsymbol{\sigma'}}\gamma^{(\boldsymbol{\sigma})}_{\boldsymbol{m},\boldsymbol{m}_1}. \qquad (43)$$

The spin-echo Ramsey contrast is given by

$$C_{\rm SE}(T) = \frac{1}{p}\left|\langle\Psi(T)|\sum_{l=1}^{N_s} {\rm e}^{{\rm i}lk_{\rm L}d}\hat{s}_{l,+}|\Psi(T)\rangle\right|. \qquad (44)$$

We vary the boson number $p$ in the range $[1, N_s - 1]$ for a lattice with $N_s = 12$ sites. The numerical results are shown in Fig. S4. We verify that the contrast is aiways one when $p = 1$. As soon as $p = 2$, we observe a significant amount of damping. To characterize quantitatively the dephasing rate, we fit the initial decay of each curve to a Gaussian function $\exp[-(\gamma_{\rm ini}T)^2]$, restricting the fit to $C_{\rm SE}(T) \geq 0.5$. The fitted curves are shown as dashed lines in Fig. S4.

* Corresponding author:fabrice.gerbier@lkb.ens.fr

[1] C. Foot, *Atomic physics* (Oxford University Press, Oxford, 2005).
[2] A. D. Ludlow, M. M. Boyd, J. Ye, E. Peik, and P. O. Schmidt, Rev. Mod. Phys. **87**, 637 (2015), URL https://link.aps.org/doi/10.1103/RevModPhys.87.637.
[3] P. Barmettler, M. Punk, V. Gritsev, E. Demler, and E. Altman, Phys. Rev. Lett. **102**, 130603 (2009), URL https://link.aps.org/doi/10.1103/PhysRevLett.102.130603.
[4] M. Babadi, E. Demler, and M. Knap, Phys. Rev. X **5**, 041005 (2015), URL https://link.aps.org/doi/10.1103/PhysRevX.5.041005.
[5] M. Vengalattore, S. R. Leslie, J. Guzman, and D. M. Stamper-Kurn, Phys. Rev. Lett. **100**, 170403 (2008), URL https://link.aps.org/doi/10.1103/PhysRevLett.100.170403.
[6] S. Hild, T. Fukuhara, P. Schauß, J. Zeiher, M. Knap, E. Demler, I. Bloch, and C. Gross, Phys. Rev. Lett. **113**, 147205 (2014), URL https://link.aps.org/doi/10.1103/PhysRevLett.113.147205.
[7] M. A. Nichols, L. W. Cheuk, M. Okan, T. R. Hartke, E. Mendez, T. Senthil, E. Khatami, H. Zhang, and M. W. Zwierlein, Science **363**, 383 (2019).
[8] A. Venegas-Gomez, A. S. Buyskikh, J. Schachenmayer, W. Ketterle, and A. J. Daley, Phys. Rev. A **102**, 023321 (2020), URL https://link.aps.org/doi/10.1103/PhysRevA.102.023321.
[9] P. N. Jepsen, J. Amato-Grill, I. Dimitrova, W. W. Ho, E. Demler, and W. Ketterle, Nature **588**, 403 (2020), ISSN 1476-4687, URL https://doi.org/10.1038/s41586-020-3033-y.
[10] P. N. Jepsen, W. W. Ho, J. Amato-Grill, I. Dimitrova, E. Demler, and W. Ketterle, Phys. Rev. X **11**, 041054 (2021), URL https://link.aps.org/doi/10.1103/PhysRevX.11.041054.
[11] S. Kolkowitz, S. L. Bromley, T. Bothwell, M. L. Wall, G. E. Marti, A. P. Koller, X. Zhang, A. M. Rey, and J. Ye, Nature **542**, 66 (2017), ISSN 0028-0836, URL http://dx.doi.org/10.1038/nature20811.
